# Supplementary material for: A carrier-wave factored one-way Navier--Stokes method for boundary-layer instability modelling
Source: arXiv:2511.12605 source file (2026-07-06)
Supplement: Supplementary file 1 [file m4p5_sm.tex]

\begin{tikzpicture}[font=\rmfamily]
\begin{axis}[
    xlabel={$\mathrm{Re}(\alpha)$},
    ylabel={$\mathrm{Im}(\alpha)$},
    xmin=-0.18, xmax=0.18,
    ymin=-0.18, ymax=0.18,
    axis lines=center,
    axis line style={-,line width=1.5pt},
    width=6cm,
    height=6cm,
    scale only axis,
    xtick=\empty,
    ytick=\empty,
    xticklabels={},
    yticklabels={},
    xlabel style={at={(axis cs:0.24,0.01)}, anchor=north east},
    ylabel style={at={(axis cs:0,0.18)}, anchor=north east},
]
% First vertical line at x = 0
% Positive part (blue with arrow)
\addplot [-{stealth}, domain=0:0.15, samples=2, blue, line width=2.5pt] coordinates {(0,0) (0,0.15)};
% Add label for the first blue arrow
\node[blue, right=2pt, font=\bfseries] at (axis cs:0,0.15) {$\alpha_{1,2,3}(\eta)$};
\node[blue, right=2pt, font=\bfseries] at (axis cs:0.1,-0.015) {$\alpha_{4,5}(\eta)$ };
\node[blue, right=2pt, font=\bfseries] at (axis cs:-0.145,0.015) {$\alpha_{4,5}(\eta)$ };

% Discrete points (more distinctive styling)
\addplot [only marks, mark=o, blue, mark size=2pt, mark options={fill=white, line width=1.8pt}] coordinates {
    (-0.05, 0.02)
    (0.06, -0.02)
};
\addplot [only marks, mark=*, red, mark size=2pt] coordinates {
    (0.0, -0.17)
    (0.0, -0.125)
    (0.0, -0.075)
    (0.0, -0.05)
};
\node[align=center, text width=6cm] (acoustic_s) at (axis cs:0.095,0.015) {\tiny{\color{black}{Downstream Acoustic S Branch}}};
\node[align=center, text width=6cm] (acoustic_f) at (axis cs:-0.095,-0.015) {\tiny{\color{black}{Downstream Acoustic F Branch}}};
% Add annotations with default font
% For discrete points
\node[align=center, text width=3cm] (mode_s) at (axis cs:0.09,-0.065) {\tiny{{\color{black}{Mode S, Downstream}}}};
\node[align=center, text width=3cm] (mode_s) at (axis cs:0.09,-0.08) {\tiny{{\color{black}{Discrete Eigenvalue}}}};
\draw[-{stealth}, line width=1.0pt, solid, gray!00!black] (axis cs:0.08,-0.055) -- (axis cs:0.065,-0.0275);

\node[align=center, text width=3cm] (mode_f) at (axis cs:-0.07,0.11) {\tiny{{\color{black}{Mode F, Downstream}}}};
\node[align=center, text width=3cm] (mode_f) at (axis cs:-0.07,0.095) {\tiny{{\color{black}{Discrete Eigenvalue}}}};
\draw[-{stealth}, line width=1.0pt, solid, gray!00!black] (axis cs:-0.06,0.08) -- (axis cs:-0.0525,0.028);

% FIXED: Removed duplicate node and fixed Viscous/Entropy Branch arrow
\node[align=center, text width=4cm] (viscous_label) at (axis cs:0.11,0.09) {\tiny{{\color{black}{Downstream Viscous/Entropy}}}};
\node[align=center, text width=4cm] (viscous_label) at (axis cs:0.09,0.077) {\tiny{{\color{black}{Branch}}}};
\draw[-{stealth}, line width=1.0pt, solid, gray!00!black] (axis cs:0.04,0.08) -- (axis cs:0.01,0.08);

% FIXED: Added two arrows pointing to the red upstream propagating discrete modes
\node[align=center, text width=4cm] (upstream_label) at (axis cs:-0.1,-0.11) {\tiny{{\color{black}{Upstream Propagating Acoustic}}}};
\node[align=center, text width=4cm] (upstream_label) at (axis cs:-0.1,-0.123) {\tiny{{\color{black}{Discrete Modes}}}};
\draw[-{stealth}, line width=1.0pt, solid, gray!00!black] (axis cs:-0.07,-0.1) -- (axis cs:-0.01,-0.055);
\draw[-{stealth}, line width=1.0pt, solid, gray!00!black] (axis cs:-0.055,-0.125) -- (axis cs:-0.01,-0.125);

% For second blue line
\addplot [-stealth, domain=0:0.1, samples=2, blue, line width=2.50pt] coordinates {(0.07,0) (0.177,0.0)};
% For red line
\addplot [-stealth, domain=0:0.1, samples=2, blue, line width=2.50pt] coordinates {(-0.07,0) (-0.177,0.0)};
%\node[align=center, text width=4cm] (mach) at (axis cs:-0.082,0.15) {$M\approx0.8$\\$\beta=0$\\$W=0$};

\node[align=center, gray!00!black] (mach) at (axis cs:0.1,-0.135) {\tiny{$M>1$}};
\node[align=center, gray!00!black] (mach) at (axis cs:0.1,-0.15) {\tiny{$\beta=0$, $W = 0$}};

\end{axis}
\end{tikzpicture}
