# Supplementary material for: A carrier-wave factored one-way Navier--Stokes method for boundary-layer instability modelling
Source: arXiv:2511.12605 source file (2026-07-06)
Supplement: Supplementary file 2 [file mp8_sm.tex]

\begin{tikzpicture}[font=\rmfamily]
\begin{axis}[
    xlabel={$\mathrm{Re}(\alpha)$},
    ylabel={$\mathrm{Im}(\alpha)$},
    xmin=-0.12, xmax=0.20,
    ymin=-0.12, ymax=0.18,
    axis lines=center,
    axis line style={-,line width=1.5pt},
    width=6cm,
    height=6cm,
    scale only axis,
    xtick=\empty,
    ytick=\empty,
    xticklabels={},
    yticklabels={},
    xlabel style={at={(axis cs:0.21,0)}, anchor=north east},
    ylabel style={at={(axis cs:0,0.18)}, anchor=north east},
]
% First vertical line at x = 0
% Positive part (blue with arrow)
\addplot [-{stealth}, domain=0:0.15, samples=2, blue, line width=2.5pt] coordinates {(0,0) (0,0.15)};
% Add label for the first blue arrow
\node[blue, right=2pt, font=\bfseries] at (axis cs:0,0.15) {$\alpha_4(\eta)$};
% Negative part (red with arrow)
\addplot [-{stealth}, domain=-0.1:0, samples=2, red, line width=2.5pt] coordinates {(0,0) (0,-0.1)};
% Add label for the red arrow
\node[red, right=2pt, font=\bfseries] at (axis cs:0,-0.1) {$\alpha_{5}(\eta)$};
% Second vertical line at x = 0.06 (blue with arrow)
\addplot [-{stealth}, domain=0:0.15, samples=2, blue, line width=2.5pt] coordinates {(0.08,0) (0.08,0.15)};
% Add label for the second blue arrow
\node[blue, right=2pt, font=\bfseries] at (axis cs:0.08,0.15) {$\alpha_{1,2,3}(\eta)$};
% Discrete points (more distinctive styling)
\addplot [only marks, mark=o, blue, mark size=2pt, mark options={fill=white, line width=1.8pt}] coordinates {
    (0.10, 0.04)
    (0.12, -0.01)
};
% Add annotations with default font
% For discrete points
\node[align=center, text width=4cm, black] (discrete_label) at (axis cs:0.10,-0.06) {\tiny{}};
\node[align=center, text width=4cm, black] (discrete_labelx) at (axis cs:0.10,-0.062) {\tiny{Downstream}};
\node[align=center, text width=4cm, black] (discrete_labelx) at (axis cs:0.10,-0.074) {\tiny{Discrete Eigenvalues}};
\draw[-{stealth}, line width=1.0pt, solid, gray!00!black] (discrete_label) -- (axis cs:0.10,0.035);
\draw[-{stealth}, line width=1.0pt, solid, gray!00!black] (discrete_label) -- (axis cs:0.117,-0.015);
\node[align=center, text width=4cm, black] (blue1_label) at (axis cs:-0.08,0.07) {\tiny{Downstream}};
\node[align=center, text width=4cm, black] (blue1_label) at (axis cs:-0.08,0.058) {\tiny{Acoustic Branch}};
\node[align=center, text width=4cm] (blue1_label2) at (axis cs:-0.098,0.08){};
\draw[-{stealth}, line width=1.0pt, solid, gray!00!black] (blue1_label2) -- (axis cs:-0.005,0.07);
% For second blue line
\node[align=center, text width=4cm, black] (blue2_label) at (axis cs:0.15,0.08) {\tiny{Downstream}};
\node[align=center, text width=4cm, black] (blue2_label) at (axis cs:0.15,0.068) {\tiny{Viscous/Entropy Branch}};
\node[align=center, text width=2.15cm] (blue2_label2) at (axis cs:0.06,0.08){};
\draw[-{stealth}, line width=1.0pt, solid, gray!00!black] (blue2_label2) -- (axis cs:0.08,0.08);
\addplot [-stealth, domain=0:0.1, samples=2, blue, line width=2.5pt] coordinates {(0.05,0) (0,0.0)};
% For red line
\node[align=center, text width=4cm, black] (red_label) at (axis cs:-0.08,-0.05) {\tiny{Upstream}};
\node[align=center, text width=4cm, black] (red_label) at (axis cs:-0.08,-0.062) {\tiny{Acoustic Branch}};
\node[align=center, text width=1.8cm] (red_label2) at (axis cs:0.00198,-0.05){};
\draw[-{stealth}, line width=1.0pt, solid, gray!00!black] (red_label2) -- (axis cs:-0.001,-0.05);
\addplot [-stealth, domain=0:0.1, samples=2, red, line width=2.50pt] coordinates {(-0.05,0) (0,0.0)};
\node[align=center, text width=4cm, black] (mach) at (axis cs:-0.082,0.125) {{\tiny{$M\approx0.8$}}};
\node[align=center, text width=4cm, black] (mach) at (axis cs:-0.082,0.11) {{\tiny{$\beta=0$, $W=0$}}};
\end{axis}
\end{tikzpicture}
